# Supplementary material for: FlexReader: Towards Adaptive Decoding Paths for Efficient Arbitrary-Length Scene Text Recognition
Source: arXiv:2610.41426 source file (2026-10-30)
Supplement: Supplementary file 1 [file a_eta.tex]

\section{eta}
